# Supplementary material for: Mesh Reconstruction from Aerial Images for Outdoor Terrain Mapping Using Joint 2D-3D Learning
Source: arXiv:2101.01844 source file (2021-04-13)
Supplement: Supplementary file 1 [file Appendix.tex]

\section{Appendix}
\label{sec:appendix}

\begin{figure*}[t]
  \centering
  \includegraphics[width=0.32\linewidth,trim=50mm 50mm 0mm 0mm, clip]{fig/baseline_sp/0021_sp_overlap.png}
  \includegraphics[width=0.32\linewidth,trim=50mm 50mm 0mm 0mm, clip]{fig/baseline_sp/0021_mesh_incomplete.png}
  \includegraphics[width=0.32\linewidth,trim=50mm 50mm 0mm 0mm, clip]{fig/baseline_sp/0021_mesh.png}
  \caption{}
  \label{fig:meshing}
\end{figure*}
